# Supplementary material for: On mission Twitter Profiles: A Study of Selective Toxic Behavior
Source: arXiv:2401.14252 source file (2024-01-25)
Supplement: Supplementary file 1 [file appendix.tex]

\clearpage
\section{Topic Extraction}
\label{sec:app_topic_modeling}

Core to our hypothesis, a Twitter profiles' disproportionately posting on a small focused set of topic(s) is a sign of possible instrumentation. To obtain topics, we leverage topic modeling on the text of individual tweets, from which the modeled topics were grouped into identifiable categories. With these categories we perform an in-depth analysis about the topics discussed in all profiles' timelines. 

\subsection{Topic modeling} is a statistical means of extracting speculative topics from a collection of documents. One approach to topic modeling on tweets is to create a single document with all the tweets of a given user \cite{mehrotra2013improving}, instead to capture better granularity in the diversity between tweets of the same user, we consider each tweet as a separate small document. To our knowledge this is the first work that applies topic modeling on 293M individual tweets. 
% \ben{If I recall did you not preform topic modelling on just a sample of all the tweets before applying it to the remainder?}\hina{I trained the model on 10\% of the tweets and then got inference for all 293M individual tweets} 
We shall discuss below the specifics of the topic modeling process performed on our dataset. 

\subsection{Contextualized topic model (CTM)} 
A \emph{topic model} extracts groups of words from given documents, the groupings are then interpreted as topics and prescribed meaning by humans. Unfortunately, the topics extracted are commonly incoherent, making human interpretation difficult. This issue is exacerbated when using short, unstructured small documents like tweets. 
Recently, neural topic models have improved topic coherence when dealing with small documents. These models use contextual embeddings %. \emph{Contextual embeddings 
such as (BERT~\cite{devlin2019bert} or ELMo~\cite{peters2017semi}) to assign a weight to a word based on the context(s) that the word was found in. 
% \ben{add a sentence on what a contextual embedding is} 
This technique have advanced the state-of-the-art neural topic models in general. For these advantages, we use the contextualized topic model (CTM) ~\cite{bianchi-etal-2021-pre}
at tweet level in this work. This model belongs to a family of neural topic models that are trained to take as an input, text embeddings and produce as an output the bag-of-words reconstruction which can be interpreted as a model.
% So, This model has two main components, the neural topic model ProdLDA ~\cite{https://doi.org/10.48550/arxiv.1703.01488}. 
% \emph{ProdLDA} is a neural topic modeling approach based on the Variational AutoEncoder (VAE). Contextualized topic models use document embeddings from SBERT (Reimers and Gurevych, 2019).
For textual embeddings we leverage, BerTweet~\cite{bertweet}, \emph{BerTweet} is a pre-trained language model for English language tweets which is trained on 850M English tweets. This model is trained using the RoBERTa pre-training procedure~\cite{https://doi.org/10.48550/arxiv.1904.09482}. \cite{conneau-etal-2020-unsupervised} shows that BerTweet is the current performance leader for small documents, outperforming baselines in NLP tasks like classification. 

We tune a pre-trained CTM model for our tweets with OCTIS (Optimizing and Comparing Topic models is Simple)~\cite{terragni-etal-2021-octis}, a useful framework for training, analyzing, and comparing topic models. \emph{OCTIS} is available as an open-source. 
% \emph{OCTIS} is available as an open-source python package used to pre-process data, run the experiments with any dataset and validate results, it gauges hyper-parameters using a Bayesian optimization approach. 
To evaluate the model performance, we opt for coherence, a standard performance evaluation metric. A \emph{Coherence} score ranges from 0 to 1, whereby larger scores indicate a strong semantic similarity between words in the resulting topics of the model, our resulting model has a coherence of 0.69.
\subsection{Topic Model Data pre-processing} 
First, (a) we filter profiles with less than 10 tweets, out of our 142,823 total users 138,430 users had more than 10 tweets. Next, (b) we filter out retweets and repeated tweets as the topic model functions better on unique documents.
Finally, (c) we generalize the tweets by converting user mentions and URLs into special tokens ``@USER'' and ``HTTPURL'', respectively.

\subsection{BERTweet textual embedding} To convert the documents to BerTweet embeddings
We first (a) tokenized a 10\% sample of tweets using ""vinai/bertweet-base" \cite{bertweet} (and preprocessed our tweets with CTM preprocessor. \cite{bianchi-etal-2021-pre}.)
During tokenization, (b) we also apply an emoji package to translate emojis into text strings, each icon was referred to as a single word token.
% An \emph{emoji} is a small digital image or icon used to express an idea or emotion. 
Capturing emojis are helpful in providing context to the accompanying text of the tweet. As per BERTweet recommendations, (c) we removed all tweets shorter than 10 or longer than 64-word tokens. For BERTweet we select a vocab size of 5000.

\subsection{Topic model Training} To train our model (a) we leverage the same randomly sampled 10\% (230,28,381 tweets) of unique tweets from the BERTweet step
% \ben{is this the same 10\% as in BERTweet?}\hina{yes}. 
% This 10\% sample was collected randomly from a pool of unique tweets by all users to train our CTM topic model.
Next, (b) we pre-process the 10\% tweet sample with ``WhiteSpacePreprocessingStopwords'' in the CTM model. The parameters used for this step are (vocabulary\_size=5000, max\_df=0.5, min\_words=2, remove\_numbers=True). Finally, (c) we use the BERTweet tokens and 10\% pre-processed tweets to train our combined topic model to extract 200 topics.

\subsection{Inferencing} We use the trained model to infer topics on the remaining tweets documents 
% with the help of a built-in CTM function "get doc topic distribution". 
For each tweet document a probability for each extracted topic (200 in our case), is produced. This is repeated for every tweet (230,283,810 total tweets) of every profile (138,430 total profiles) we call these the "Topic probability distribution vectors". 

% From our investigation, this also is the biggest dataset of tweets to date that have used contextualized topic model and BERTweet embeddings topic modeling combination on this scale. \ben{what is the next largest use of tweets?}\hina{That we have the perspective score for each tweet in the dataset.}\ben{as in from other works, if we are the largest give an example of another work + citation using a large amount.}

\subsection{Hardware} The topic models were trained and inference completed on an Amazon ec2 g4dn.8xlarge, a GPU instance with 32vCPUs, 128GB memory and 1 GPU. It took 32 days from start to end to complete topic modeling on our dataset.
% \ian{Most of these details belong in the appendix - here only a very brief overview of which model was used and the main parameter settings.}

\subsection{Understanding the resulting Learned Topics} % Data visualization using pyLDAvis
\label{sec:pyldavis}
% \ben{This entire subsubsection is a bit too specific to Topic 8, and no discussion on the general bubble plot has been made, likely can be pushed to the appendix, or cut.}\hina{I suggest we push it to an appendix, The idea to add this part was to be transparent about how we interpreted topics because the group's selection is based on it.}\ian{The details of LDAvis are not necessary - just very briefly what it does (a sentence or two). Fig 2 seems supurfluous. This should be a subsection "Topic Model Evaluation". A single example tweet here in the main body is enough, and we can provide further examples in the appendix.}

To provide visually accessible interpretations of the topic modeling results we leverage LDAvis~\cite{pylDAvis}, \emph{LDAvis} provides metrics to gauge differences between topics.
We interpreted topic by "most relevant terms per topic", LDAvis defines the relevance of a term "w" in a topic "k" to be determined by a weight parameter $\lambda$; where 0 <= $\lambda$ <= 1 as expressed in Eq: \ref{eq:1}~\cite{pylDAvis}:
\begin{equation}
\label{eq:1}
r(w, k \mid \lambda)=\lambda \log \left(\phi_{k w}\right)+(1-\lambda) \log \left(\frac{\phi_{k w}}{p_{w}}\right)
\end{equation}
where $\lambda$ determines the weight given to the probability of term "w" under topic "k" relative to its lift (by measuring both on the log scale). With trial and error on the relevance parameter, we set  $\lambda$ = 0, to rank the top 30 most relevant terms in a topic solely by their lift.

\begin{table}[h]
\centering
\resizebox{0.5\textwidth}{!}{
% \tabcolsep=0.08cm
% {\begin{tabular}{p{1.15cm}|p{8.15cm}|p{1.15cm}|p{1.15cm}} 

\begin{tabular}{l|p{3.95cm}|c|c}
\toprule
{\bf Group} & {\bf Tweet} &{\bf Tweet Tox.} &{\bf Tweet category} \\\hline
{\bf Gp-II}& \texttt{Covid policies \& Nursing Home are to blame for this. They KNEW that 20yr old was psych ward for Schizophrenia. But bcz he got CV19 they fuckin moved nigga to nursing home, in accordance with failed policy.} &0.9&Health/Covid\\\hline
{\bf Gp-III}& \texttt{He's just another illegitimate skank. \#FuckJoeBiden \#BidenCrimeFamily \#NotADoctor}&0.9&Politics\\\hline
{\bf Gp-IV}& \texttt{``What a nasty dual face tactics! you guys Trump has arrived at the Georgia World Congress Center for remarks at a Black Voices for Trump. campaign rollout.''}&0.9&Politics\\\hline
{\bf Gp-V}& \texttt{I bet crises looks for these MFs!! \#fucktrump, \#fuckMAGA}&0.9&Politics\\\hline
% {\bf Group-VII} & {\bf Tweet} &{\bf Topic No.} &{\bf Toxicity Score} \\\hline
{\bf Gp-VI}& \texttt{My a**! Black lives are fucked, we in constant danger, ya keep buzz doing nothing, sayin MAGA MAGA MAGA !}&0.9&News/blogs\\\hline
{\bf Gp-VII}& \texttt{\'Deeply disturbing\': Feds did not charge extremists in domestic terror plot to kidnap the nigg, what a snitch government allows this?}&0.9&News/blogs\\\hline

{\bf Gp-VIII} &    \texttt {I think the announcement broke Trump's brain. What does this even mean? Fukcing idiotic ways to react...}   &  0.9& Politics\\

\bottomrule  
\end{tabular}
}
\caption{Example most toxic tweets from manually validated on-mission Twitter profiles from Groups II-VII and an example tweet from on-mission profile(ground truth). Profiles IDs are not shared as per Twitter regulations and user privacy. The toxicity score of the tweet is provided by the Perspective API, and the category comes from the tweet topic probability score and category of the respective topic. 
% \ik{Are Profile A belongs to Group VI and Group VII? If not then use different labels for the column.\hina{different groups}} 
% have similar table for not-on-mission profiles?}
% \vspace{-5mm}
\label{tab:classifier_Example}}
\end{table}
